# Supplementary material for: Conceptual Organization is Revealed by Consumer Activity Patterns
Source: arXiv:1810.08577 source file (2018-10-19)
Supplement: Supplementary file 2 [file supp.tex]

@article{Blei2003,
abstract = {We describe latent Dirichlet allocation (LDA), a generative probabilistic model for collections of discrete data such as text corpora. LDA is a three-level hierarchical Bayesian model, in which each item of a collection is modeled as a finite mixture over an underlying set of topics. Each topic is, in turn, modeled as an infinite mixture over an underlying set of topic probabilities. In the context of text modeling, the topic probabilities provide an explicit representation of a document. We present efficient approximate inference techniques based on variational methods and an EM algorithm for empirical Bayes parameter estimation. We report results in document modeling, text classification, and collaborative filtering, comparing to a mixture of unigrams model and the probabilistic LSI model.},
archivePrefix = {arXiv},
arxivId = {1111.6189v1},
author = {Blei, David M; and Ng, Andrew Y; and Jordan, Michael I;},
doi = {10.1162/jmlr.2003.3.4-5.993},
eprint = {1111.6189v1},
isbn = {9781577352815},
issn = {15324435},
journal = {Journal of Machine Learning Research},
pages = {993--1022},
pmid = {21362469},
title = {{Latent Dirichlet Allocation}},
volume = {3},
year = {2003}
}
@inproceedings{Taddy2012,
abstract = {Topic modeling is a mixed-membership framework for dimension reduction that is widely applied in text-mining, among other areas. This article describes an algorithm for posterior maximization under such models, identifying computational and conceptual gains that come from working with an alternative model parameterization. We then show that fitted parameters can be used as the basis for a novel approach to marginal likelihood estimation, founded on block-diagonal approximation to the information matrix, that facilitates choosing the number of latent topics. This likelihood-based model selection is complemented with a goodness-of-fit analysis built around estimated residual dispersion. We survey existing estimation methodology, emphasizing aspects that motivated us to develop new techniques, and examples are provided to illustrate model selection as well as to compare our estimation against standard variational approximations.},
archivePrefix = {arXiv},
arxivId = {arXiv:1109.4518v3},
author = {Taddy, Matthew a},
booktitle = {Proceedings of the Fifteenth International Conference on Artificial Intelligence and Statistics (AISTATS 2012)},
eprint = {arXiv:1109.4518v3},
file = {:Users/adamhornsby/Documents/University/PhD/Projects/LDA/papers/taddy12.pdf:pdf},
issn = {15337928},
number = {2003},
pages = {1184--1193},
title = {{On Estimation and Selection for Topic Models}},
year = {2012}
}
@article{Chang2009,
abstract = {Probabilistic topic models are a popular tool for the unsupervised analysis of text, providing both a predictive model of future text and a latent topic representation of the corpus. Practitioners typically assume that the latent space is semantically meaningful. It is used to check models, summarize the corpus, and guide exploration of its contents. However, whether the latent space is interpretable is in need of quantitative evaluation. In this paper, we present new quantitative methods for measuring semantic meaning in inferred topics. We back these measures with large-scale user studies, showing that they capture aspects of the model that are undetected by previous measures of model quality based on held-out likelihood. Surprisingly, topic models which perform better on held-out likelihood may infer less semantically meaningful topics.},
archivePrefix = {arXiv},
arxivId = {arXiv:1011.1669v3},
author = {Chang, Jonathan and Gerrish, Sean and Wang, Chong and Blei, David M},
doi = {10.1.1.100.1089},
eprint = {arXiv:1011.1669v3},
file = {:Users/adamhornsby/Library/Application Support/Mendeley Desktop/Downloaded/Chang et al. - 2009 - Reading Tea Leaves How Humans Interpret Topic Models.pdf:pdf},
isbn = {9781615679119},
issn = {1098-6596},
journal = {Advances in Neural Information Processing Systems 22},
pages = {288----296},
pmid = {25246403},
title = {{Reading Tea Leaves: How Humans Interpret Topic Models}},
url = {http://www.umiacs.umd.edu/{~}jbg/docs/nips2009-rtl.pdf},
year = {2009}
}
@article{Sievert2014,
abstract = {We present LDAvis, a web-based interactive visualization of topics estimated using Latent Dirichlet Allocation that is built using a combination of R and D3. Our visualization provides a global view of the topics (and how they differ from each other), while at the same time allowing for a deep inspection of the terms most highly associated with each individual topic. First, we propose a novel method for choosing which terms to present to a user to aid in the task of topic interpretation, in which we define the relevance of a term to a topic. Second, we present results from a user study that suggest that ranking terms purely by their probability under a topic is suboptimal for topic interpretation. Last, we describe LDAvis, our visualization system that allows users to flexibly explore topic-term relationships using relevance to better understand a fitted LDA model.},
archivePrefix = {arXiv},
arxivId = {arXiv:1011.1669v3},
author = {Sievert, Carson and Shirley, Kenneth},
doi = {10.1.1.100.1089},
eprint = {arXiv:1011.1669v3},
file = {:Users/adamhornsby/Documents/University/PhD/Projects/LDA/papers/sievert-illvi2014.pdf:pdf},
isbn = {1932432655},
issn = {10495258},
journal = {Proceedings of the Workshop on Interactive Language Learning, Visualization, and Interfaces},
pages = {63--70},
pmid = {25246403},
title = {{LDAvis: A method for visualizing and interpreting topics}},
url = {http://www.aclweb.org/anthology/W/W14/W14-3110},
year = {2014}
}
